# Supplementary material for: Repeat After Me: Transformers are Better than State Space Models at Copying
Source: arXiv:2402.01032 source file (2024-06-03)
Supplement: Supplementary file 1 [file additional_experiments.tex]

\section{Positional Embeddings}

\begin{figure*}[t]

\begin{subfigure}{0.495\textwidth}%0.33
 \hspace{-.1cm}
 \includegraphics[width=.9\linewidth]{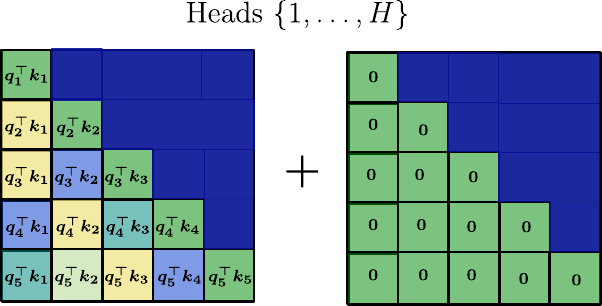}\label{fig:nope}
 
% \vspace*{-.4cm}
 
 \caption{}\label{fig:add_ape}
\end{subfigure}
\hspace{.1cm}
\begin{subfigure}{0.495\textwidth}%0.33
\hspace{1cm}
 \includegraphics[width=1.\linewidth]{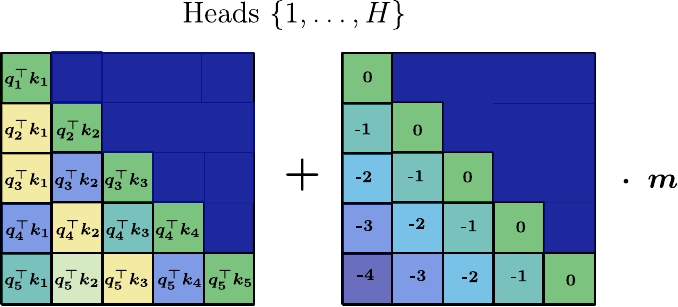}
 
% \vspace*{-.4cm}
 
 \caption{}\label{fig:alibi}
\end{subfigure}

\begin{subfigure}{1\textwidth}
\includegraphics[width=1.05\linewidth]{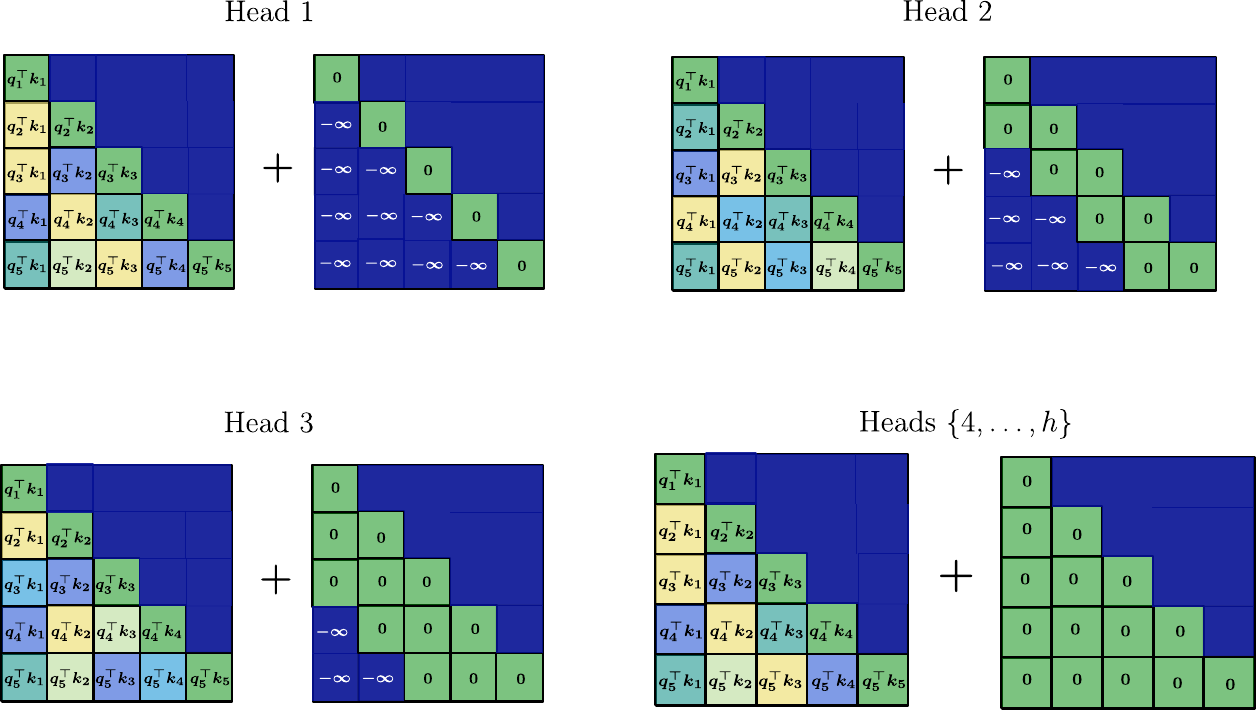}
\caption{}\label{fig:hard_alibi}
\end{subfigure}
\caption{\small }
%\vspace{-.5cm}
\end{figure*}

\section{Additional Experiments}

\begin{figure}
    \centering
    \includegraphics{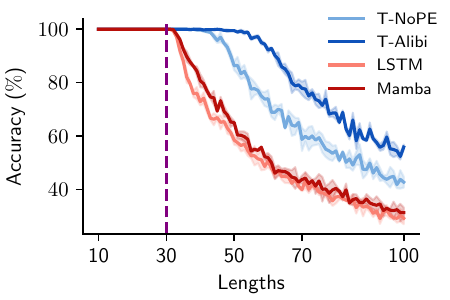}
    \caption{Induction Infinite}
    \label{fig:induction_infinite}
\end{figure}

\begin{figure}
    \centering
    \includegraphics{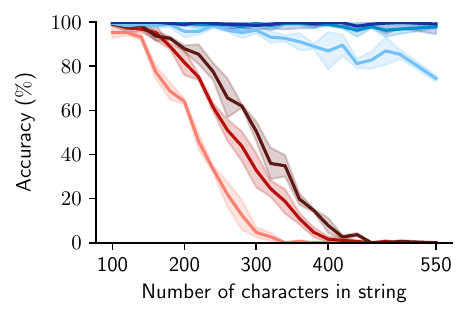}
    \caption{\textbf{TODO: move to Appendix, add c4 figure}}
    \label{fig:pretrained}
\end{figure}

\begin{figure}
    \centering
    \includegraphics{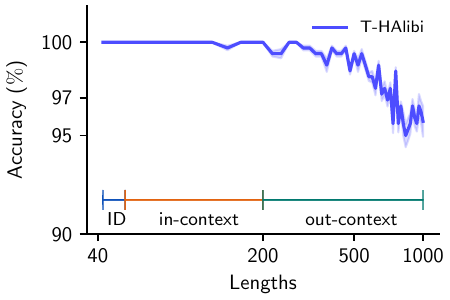}
    \caption{Caption}
    \label{fig:out_distribution}
\end{figure}
